# Supplementary material for: DeepVisualInsight: Time-Travelling Visualization for Spatio-Temporal Causality of Deep Classification Training
Source: arXiv:2201.01155 source file (2021-12-31)
Supplement: Supplementary file 1 [file appendix.tex]

\section{Appendix}
